# Supplementary material for: A comparative study of star formation processes in different environments
Source: arXiv:0908.4285 source file (2009-08-28)
Supplement: Supplementary file 1 [file appendixA.tex]

\appendix
\chapter{Temperature and abundance variations}

At the end of the 60s and beginning of the 70s, Peimbert
\cite*{1967ApJ...150..825P}, Peimbert and Costero \cite*{1969BOTT....5....3P},
and Peimbert \cite*{1971BOTT....6...29P} established a 
complete analytical formulation to study the discrepancies between the
abundances relative to hydrogen derived from RLs and CELs when a constant electron
temperature is assumed. These discrepancies have been observed in a great sample
of galactic and extragalactic \HII regions and planetary nebulae 
(see Peimbert et al., 2000; Peimbert, 2003; Peimbert and Peimbert, 2003;
Tsamis et al., 2003; Esteban et al., 2004; Peimbert et al., 2005; Garc\'ia-Rojas et al., 2005; 
Garc\'ia-Rojas et al., 2006; Garc\'ia-Rojas et al., 2007; Guseva et al., 2006; Guseva et al.,
2007; Rubin et al., 2002; Wesson et al., 2005; Liu et al., 2006; Liu, 2006;
Peimbert and Peimbert, 2006, and references therein).
\nocite{2004MNRAS.355..229E,2005MNRAS.362..301G,2006MNRAS.368..253G,2007ApJ...670..457G,2000ApJ...541..688P,2003ApJ...584..735P,2003MNRAS.338..687T,2003RMxAC..16..113P,2005ApJ...634.1056P,2006ApJ...644..890G,2007A&A...464..885G,2002MNRAS.334..777R,2005MNRAS.362..424W,2006MNRAS.368.1959L,2006IAUS..234..219L,2006IAUS..234..227P}
In the first of these original works, Peimbert proposed that this discrepancy
is due to spatial temperature variations which can be characterized by two
parameters, the average temperature weighted by the square of the density over
the volume considered, T$_0$, and the root mean square temperature
fluctuation, t$^2$. They are given by:

\begin{eqnarray}
\label{t0}
T_0(X^{i+})\,=\,\frac{\int T_e\,N_e\,N(X^{i+})\,dV}{\int N_e\,N(X^{i+})\,dV}
\end{eqnarray}

\noindent
and

\begin{eqnarray}
\label{t2}
t^2(X^{i+})\,=\,\frac{\int(T_e-T_0(X^{i+}))^2\,N_e\,N(X^{i+})\,dV}{T_0(X^{i+})^2\int N_e\,N(X^{i+})\,dV}
\end{eqnarray}

\noindent
where N$_e$ and N$(X^{+i}$) are the local electron and ion densities
of the observed emission lines, respectively, 
T$_e$ is the local electron temperature and $V$ is the observed volume
\cite{1967ApJ...150..825P}.  These are equation (9) and (12), respectively, of
that work.

It is possible to obtain the values of T$_0$ and t$^2$ using different
methods. One possibility is compare the electron temperatures obtained using two
independent ways,
generalmente se utilizan temperaturas que se originan en distintas zonas de la
nebulosa, una que represente a las zonas mas calientes y otra a las mas frias.
Notemos que las lineas excitadas colisionalmente tienen mayor intensidad cuando
las temperaturas son mas altas, comportamiento inverso al que tienen las lineas
de recombinacion que son mas intensas cuando T es menor.
Cuando no tenemos temperaturas derivadas de las lineas de recombinacion podemos
utilizar en su lugar las temperaturas derivadas a partir de las
discontinuidades, como por ejemplo las de Balmer y la de Paschen del hidrogeno.

Otra manera de determinar cuales deben ser los valores de T$_0$ y de t$^2$ es
comparar las abundancias obtenidas for a particular ion from the CELs and RLs.
The first is calculated from the observed forbidden
lines, para el atomo i+1 veces ionizado,
cuya mayor contribucion es colisional, mientras que las segundas se determinan a
partir de las recombinaciones observadas, para el atomo i veces
ionizado. Debemos ver cuales son esos valores que hacen que las abundancias
calculadas de esas dos maneras distintas sean las mismas.
The proper line temperatures for 
CELs and RLs, T$_{CEL}$ and T$_{RL}$, respectively, for t$^2\ll1$, ($\Delta
E_{CEL}$/kT$_0$-1/2)\,$\neq$\,0, and $\alpha$\,$\neq$\,0 are given by equations
(20) and (22) of Peimbert and Costero \cite*{1969BOTT....5....3P}:

\begin{eqnarray}
\label{tcel}
T_{CEL}\,=\,T_0\,\Big\{1+\Big[\frac{(\Delta E_{CEL}/kT_0)^2-3\Delta E_{CEL}/kT_0+3/4}{\Delta E_{CEL}/kT_0-1/2}\Big]\frac{t^2}{2}\Big\}
\end{eqnarray}

\noindent
and

\begin{eqnarray}
\label{trl}
T_{RL}\,=\,T_0\Big[1-(1-\alpha)\frac{t^2}{2}\Big]
\end{eqnarray}

\noindent where $\alpha$ is the power of the temperature for a given
recombination line and $\Delta E_{CEL}$\,=\,$\Delta E_{mn}$ is the energy
difference, in eV, between the two levels (m and n are the upper and lower
levels, respectively) of the atomic transition that produces the line that we
have used to calculate the ionic abundace. 

From equation (15) of Peimbert \cite*{1967ApJ...150..825P} the derived temperature from the
ratio of emission line fluxes is related to the average temperature, whether
$\Delta E\neq\Delta E^{\ast}$ and t$^2\ll1$, by

\begin{eqnarray}
\label{tlamb}
T(\lambda_{mn}/\lambda_{m'n'})\,=\,T_0\Big[1+\Big(\frac{\Delta E+\Delta E^{\ast}}{kT_0}-3\Big)\frac{t^2}{2}\Big]
\end{eqnarray}

\noindent where $\Delta E$ and $\Delta E^{\ast}$ represent the differences in
energy between the two levels of the atomic transitions that produce the lines
that we have used to derive the temperature. For example, the equation for
T([O{\sc iii}]) involves the energy differences for the
three lines that we have used to calculate it, $\lambda\lambda$\,4363,
4959, and 5007\,\AA. 

Cuando calculamos las abundancias con sus respectivas temperaturas derivadas a
partir de las lineas de emision sin tener en cuenta las diferencias en las
mismas producidas por las fluctuaciones de temperatura, cuando estas esten
presentes,  habra un error en el
calculo de las abundancias. De los trabjos de Peimbert 1967, 1969 y  ruiz 2003
se obtiene la siguiente ecuacion para calcular en cociente de dos iones
cualquiera de dos elementos cualquiera a partir del cociente de abundancias
calculada con t$^2$ igual a 0:

\begin{eqnarray}
\label{abvar}
\lefteqn{\Big[\frac{N_{CEL}(X^{+i})}{N_{RL}(Y^{+j})}\Big]_{t^2>0}\,=\,
  \frac{T_{RL}^{\alpha}T_{CEL}^{0.5}}{T(\lambda_{mn}/\lambda_{m'n'})^{\alpha+0.5}}
{} } \nonumber\\ & & {}  
\times\,exp\Big[-\frac{\Delta E_{CEL}}{k\,T(\lambda_{mn}/\lambda_{m'n'})}+\frac{\Delta
  E_{CEL}}{k\,T_{CEL}}\Big]\,\times\,\Big[\frac{N_{CEL}(X^{+i})}{N_{RL}(Y^{+j})}\Big]_{t^2=0}  {}
\end{eqnarray}

\noindent where T($\lambda_{mn}/\lambda_{m'n'}$) is the temperature adopted to
calculate the abundance for each ion.

En el caso particular en el que tenemos un mismo atomo y tomamos el ion i+1 para
el CEL y el i para el RL, y obtenemos un cociente para las abundancias
calculadas para t$^2$ igual a cero es menor a uno, entonces suponemos que
existen fluctuaciones de temperatura, las cuales pueden ser calculadas haciendo
que esta ecuacion sea igual a 1, en el caso particular
que Y$^{+j}$ sea igual a X$^{(i-1)+}$, y teniendo en cuenta las ecuaciones
(\ref{tcel}), (\ref{trl}), and (\ref{tlamb}).

We have followed the works by Peimbert et al.\ (2000), Peimbert et al.\
(2002), Peimbert et al.\ (2004) and Ruiz et al.\ (2003)
\nocite{2000ApJ...541..688P,2002ApJ...565..668P,2004ApJS..150..431P,2003ApJ...595..247R}
to derived the values of T$_0$ and t$^2$ for our WHT 
spectra. In our particular case, we can not estimate the temperature
fluctuations from the RL/CEL abundance ratio in any case, since we could not
measure with good enougth  precision the observed fluxes from CELs and RLs for
the corresponding ions (X$^{(i+1)+}$ and X$^{i+}$, respectively). We only can
derive the temperature fluctuations combining the Balmer temperature and same of
the derived temperatures within the different temperature schemes, which we
describe in the next paragraphs.

\section*{One-zone ionization scheme}

This scheme supposes that one temperature is representative of the whole nebula 
and derived the chemical abundances using it. This temperature can be, for
example, T([O{\sc iii}]) (see Garc\'ia-Rojas et al., 2004, and references
therein). \nocite{2004ApJS..153..501G} Then, combining this  
temperature and one calculated from RLs, such as T(Bac), and using equations
(\ref{tlamb}) and (\ref{trl}), we have a system of two equations to find T$_0$
and t$^2$. For example, combining T([OIII]) and T(Bac), given

\begin{eqnarray}
\label{toiii}
T([O\textrm{\sc iii}])\,=\,T_0\,\Big[1+\frac{1}{2}\Big(\frac{90800}{T_0}-3\Big)\,t^2\Big]
\end{eqnarray}

\noindent
and

\begin{eqnarray}
\label{tbac}
T(Bac)\,=\,T_0\big(1-1.67t^2\big)
\end{eqnarray}

Moreover, se pueden determinar otros valores para T$_0$ y t$^2$ haciendo
coincidir las abundancias determinadas a partir de las CELs y las RLs para un
mismo ion, y utilizando como T($\lambda_{mn}/\lambda_{m'n'}$) la misma
temperatura representativa con la que calculamos las abundancias. Para esto se
utilizan las ecuaciones (\ref{tcel}), (\ref{trl}), (\ref{tlamb}), and
(\ref{abvar}), esta ultima igualada a 1.

En el limite de bajas densidades y profundidas optica pequeña, y para t$^2$ mucho
menor que 1, de la ecuacion (14) de Peimbert (1967), la temperatura electronica
para el helio es proporcional a $<alpha>$, the average value of the power of the
temperature for the helium lines utilizadas para calcular las abundancias
ionicas del He+ respecto a H+, and $\beta$ is the power of the spectrum for
H$\beta$, para alpha distinto de $\beta$, given

\begin{eqnarray}
\label{the}
T(He\textrm{\sc ii})\,=\,T(He\textrm{\sc ii},H\textrm{\sc ii})\,=\,T_0\Big[1+\big(\langle\alpha\rangle+\beta-1\big)\frac{t^2}{2}\Big]
\end{eqnarray}

\noindent The value of the power of the temperature for each helium line in the
low density limit have been obtained from Benjamin et al.\
\cite*{1999ApJ...514..307B} and the value  for H$\beta$  has been obtained
from Storey and Hummer \cite*{1995MNRAS.272...41S} and it is equal to -0.89. 
$\langle\alpha\rangle$ is the average weighted according to the observational errors
\cite{2000ApJ...541..688P}. In our case, for each
WHT spectrum, we have obtained $\langle\alpha\rangle$ equal to -1.37, -1.42, and -1.43
for SDSS J002101.03+005248.1, SDSS J003218.59+150014.2, and SDSS
J162410.1-002202.5, respectively.

Debemos tener en cuenta que si pudieramos obtener de manera independiente el
valor de la temperatura de He podriamos utilizarlo para derivar otra estimacion
de T$_0$ y t$^2$ combinando las ecuaciones (\ref{toiii}) y (\ref{the}), o sea
relacionando T(OIII) con T(HeII) de la
misma manera que lo hicimos entre la primera y T(Bac).

Posteriormente se puede realizar un promedio pesado con los errores de los
distintos valores obtenidos para T$_0$ y t$^2$, los cuales van a ser utilizados
cuando recalculemos las abundncias.

Furthermore, from equation (\ref{trl}), we can calculate the temperature for
H$\beta$, T(H$\beta$):

\begin{eqnarray}
\label{thbeta}
T(H\beta)=T_0\Big[1-0.95\,t^2\Big]
\end{eqnarray}

\noindent where the value of the power of the temperature for H$\beta$ 
is the same as in the previous equation. 
This temperature is necessary to recalculate the ionic abundances relatine to
hydrogen for t$^2$ greater than zero [see equation (\ref{abvar})].

\section*{Two-zone ionization scheme}

Este esquema utiliza dos temperaturas distintas. Una representa a la zona de
baja exccitacion y la otra a la de alta. Por ejemplo, se puede utilizar la
temperatura de [OII] o de [NII] para calcular las abundancias relativas al
hidrogeno de los iones de baja excitacion, como por ejemplo O+, S+, y N+, y la
temperatura de [OIII] o de [SIII] para los iones de alta excitacion, tales como
O2+, S2+, Ne2+, Ar2+, y Fe2+.

Following the paper by Peimbert et al.\ \cite*{2002ApJ...565..668P} we have
taken, as example, T([O{\sc ii}]) and T([O{\sc iii}]) as the temperatures
which represent the low- and high-ionization zones. Peimbert
\cite*{2003ApJ...584..735P} used the temperature 
derived from the ratio of [N{\sc ii}] $\lambda\lambda$5755 and 6584 lines,
T([N{\sc ii}]), for the low ionization zone. En este caso tendremos T$_{02}$ y
T$_{03}$, las temperaturas medias de O+ y O2+, respectivamente. Estas estan
dadas por la ecuacion (\ref{t0}) para N(O+) y N(O2+), respectivamente
(see equations (8) and (9) from Peimbert et al., 2002).
\nocite{2002ApJ...565..668P} Esta vez el
oxigeno esta presente en la forma de O+ y O++, con el peso de O+ descripto por
el parametro $a(O^+,O^{2+})\,=\,a$ definido en la ecuacion (7) de ese mismo
trabajo:

\begin{eqnarray}
\label{eca}
a(O^+,O^{2+})\,=\,a\,=\frac{\int N_eN(O^+)dV}{\int N_eN(O^+)dV+\int N_eN(O^{2+})dV}
\end{eqnarray}

\noindent where N(O$^+$) and N(O$^{2+}$) are given by the derived abundances.
Then, the average temperature for the whole ionized region, T$_0$, can be
written as a function of $a$ in the the following way
(equation (10) of Peimbert et al., 2002)
\nocite{2002ApJ...565..668P}

\begin{eqnarray}
\label{ecb}
T_0\,=\,a\,T_{02}+(1-a)\,T_{03}
\end{eqnarray}

Then, they define the parameter $b$, the fractional difference between T$_03$ and
T$_0$ as

\begin{eqnarray}
\frac{T_{03}}{T_0}\,=\,1+b
\end{eqnarray}

\noindent equation (11) of Peimbert et al.\ \cite*{2002ApJ...565..668P}.

In general there are not a uniform temperature inside each zone, and their
temperature fluctuations (t$^2_2$ and t$^2_3$ for the low- and
high-ionization zone, respectively) are give by equation (\ref{t2}) with the
corresponding values for T$_0$ and N(X$^i$). In this example, T$_{02}$ and
N(O$^+$) for t$^2_2$, and T$_{032}$ and N(O$^{2+}$) for t$^2_3$ 
(see equations (13) and (14) from Peimbert et al., 2002).
\nocite{2002ApJ...565..668P}

The mean square temperature fluctuation for the entire HII region, t$^2$, is
given by the difference in temperature between each zone and the average for
the whole HII region and the additional contribution due to inhomogeneities in
each zone.  Taking into account equations (\ref{eca}) and (\ref{ecb}) they
obtained in their equation (16) that the mean square temperature variations in
the entire volume of the ionized nebula is given by

\begin{eqnarray}
t^2\,=\,b^2\Big(\frac{1-a}{a}\Big)+at^2_2+(1-a)t^2_3
\end{eqnarray}

From equation (\ref{tlamb}) it is possible to relate  T([O{\sc ii}]) and
T([O{\sc iii}]) with their corresponding average temperatures and mean square
temperature variations through these two equations:

\begin{eqnarray}
\label{toii}
T([O\textrm{\sc ii}])\,=\,T_{02}\,\Big[1+\frac{1}{2}\Big(\frac{97300}{T_{02}}-3\Big)\,t^2_2\Big]
\end{eqnarray}

\noindent
and 

\begin{eqnarray}
\label{toiii2}
T([O\textrm{\sc iii}])\,=\,T_{03}\,\Big[1+\frac{1}{2}\Big(\frac{90800}{T_{03}}-3\Big)\,t^2_3\Big]
\end{eqnarray}

\noindent equations (18) and (17), respectively, of Peimbert et al.\
\cite*{2002ApJ...565..668P}. Then, they derive an equation which has the same 
physical meaning as that of this two last ones and it relates T$_0$ and t$^2$
with temperatures that can be calculated from the observations, such as T([O{\sc
    ii}]) and T([O{\sc iii}]). The derivation of this equation, under the
assumption that t$^2_2$\,$\approx$\,t$^2_3$ and keeping the equations to second
order in the temperature variations ($b$,t$_2$,t$_3$, and t), is given in the
Appendix of the work by Peimbert et al.\ \cite*{2002ApJ...565..668P}, and it is

\begin{eqnarray}
\label{toiioiii}
T([O\textrm{\sc ii}]+[O\textrm{\sc iii}])\,=\,T_{0}\,\Big[1+\Big(\frac{\theta}{T_{0}}-3\Big)\,\frac{t^2}{2}\Big]
\end{eqnarray}

\noindent or

\begin{eqnarray}
\label{toiioiii2}
T_{0}\,=\,T([O\textrm{\sc ii}]+[O\textrm{\sc iii}])\Big[1-\Big(\frac{\theta}{T([O\textrm{\sc ii}]+[O\textrm{\sc iii}])}-3\Big)\,\,\frac{t^2}{2}\Big]
\end{eqnarray}

\noindent where $\theta$ represents an effective average over the excitation
energy needed to produce these forbidden oxygen lines (equation (20)
of  Peimbert et al., 2002).

\begin{eqnarray}
\label{theta}
\theta\,=\,97300\,a+90800\,(1-a)
\end{eqnarray}

\noindent and T([O{\sc ii}]+[O{\sc iii}]) is an average of these two
temperatures, but it is not a simple average weighted by the factors $a$ and
$(1-a)$, it needs a factor $\Gamma$ (see Appendix of Peimbert et al., 2002) 
to be accurate to second order and which represents the second-order correction
due to the difference in temperature between the low- and high-ionization
zones. Then, T([O{\sc ii}]+[O{\sc iii}]) is given by equation (21) or (A1) of
that work in this form

\begin{eqnarray}
\label{toiioiii3}
T([O\textrm{\sc ii}]+[O\textrm{\sc iii}])\,=\,\big[aT([O\textrm{\sc ii}])\,+\,(1-a)T([O\textrm{\sc iii}])\big]\Gamma
\end{eqnarray}

\noindent and

\begin{eqnarray}
\label{Gamma}
\Gamma\,=\,1+\delta^2\gamma
\end{eqnarray}

\noindent where $\delta$ is the relative difference between these two
temperatures and the free parameter $\gamma$ is used to recover the physical
meaning of equations (\ref{toii}) and (\ref{toiii2}), then (see equations
  (A3) and (A7) of  Peimbert et al., 2002)

\begin{eqnarray}
\label{delta}
\delta\,=\,\frac{T([O\textrm{\sc iii}])}{T([O\textrm{\sc ii}])}-1
\end{eqnarray}

\noindent and

\begin{eqnarray}
\label{gamma}
\gamma\,=\,\frac{1}{2}(1-a)\,a\Big[\Big(\frac{\theta}{T_0}\Big)-3\Big] 
\end{eqnarray}

\noindent Note that the factor $\Gamma$ is very close to one when
$a\,(1-a)\,<\,$0.08 or  0.9\,$<$\,T([O{\sc ii}])/T([O{\sc iii}])\,$<$\,1.1. In
these particular cases, equations  (\ref{eca}), (\ref{theta}), and (\ref{toiioiii3}) 
are only needed to derive T([O{\sc ii}]+[O{\sc iii}]) from the observed
temperatures. If $\Gamma$ is larger than one, equations (\ref{Gamma}),
(\ref{delta}), and (\ref{gamma}) are also needed \cite{2002ApJ...565..668P}.

Then, in the same way that in the one-ionization scheme, we can combine the
equation (\ref{tbac}) for T(Bac) with equation (\ref{toiioiii}) or
(\ref{toiioiii2}) to obtain T$_0$ and t$^2$. We can use equations (\ref{the})
and (\ref{thbeta}) in the same way as in the first scheme to calculate T(He{\sc
  ii}) and T(H$\beta$) from the derived T$_0$ and t$^2$, and, in the case that
we can estimate T(He{\sc ii}) from and independent method, we can take another
estimation of T$_0$ and t$^2$.

%being $\delta$\,=\,$b/a$ since to first order T([O{\sc ii}])\,=\,T$_{02}$
%and T([O{\sc iii}])\,=\,T$_{03}$, they deduce 

%\noindent
%The solution of this system of equations for each galaxy are listed in table
%\ref{fluc}. We have to note that ....  en dos de los casos los valores de t2 son
%practicamente nulos

\begin{table}
{\small
\caption{T$_0$ and t$^2$ parameters}
\label{fluc}
\begin{center}
\begin{tabular}{l c c }
\hline
\hline
       name               &     T$_0$         &   t$^2$         \\
\hline
SDSS J002101.03+005248.1  &    1.24$\pm$0.37  &   0.005$\pm$0.045  \\
SDSS J003218.59+150014.2  &    1.08$\pm$0.24  &   0.069$\pm$0.029  \\
SDSS J162410.1-002202.5   &    1.24$\pm$0.31  &   0.001$\pm$0.039  \\
\hline

\multicolumn{3}{l}{T$_0$ in 10$^4$\,K}

\end{tabular}

\end{center}
}
\end{table}

%\noindent the results for T(H$\beta$) and their errors are listed in table
%\ref{temden}. 

%The results for T(He{\sc ii}) and their correspondeing errors are listed in
%table \ref{temden}.

\section*{Abundance variations}
\label{abunvar}

To recalculate the ionic abundaces we have used the ecuation (26) of the work
by Peimbert and Costero \cite*{1969BOTT....5....3P}, rewritten in the same
ways as ecuation (14) of Peimbert et al.\ \cite*{2004ApJS..150..431P}

\begin{eqnarray}
\Big[\frac{N_{CEL}(X^{+i})}{N(H^{+})}\Big]_{t^2>0}\,=\,
  \frac{DT(H\beta)^{\alpha}}{CT(\lambda_{mn})^{-0.5}}\,\times\,
  exp\Big[-\frac{\Delta
  E}{k\,T(\lambda_{mn})}\Big]\,\frac{I(X^{+i},\lambda_{mn})}{I(H\beta))}  
\end{eqnarray}

\noindent where $I(X^{+i},\lambda_{mn})$ and $I(H\beta)$ are the observed
emission flux for the forbidden and H$\beta$ lines, respectively, $\lambda_{mn}$
is the wavelength associated with this forbidden emission line, and C and D are
obtained from atomic computations. When t$^2$ is equal to zero,
T(H$\beta$)\,=\,T($\lambda_{mn}$)\,=\,T([O{\sc iii}]). In general,
T($\lambda_{mn}$) is give by equation (\ref{tcel})
(T($\lambda_{mn}$)\,$\equiv$\,T$_{CEL}$).

For t$^2$ greater than zero we have derived the chemical abundances using the
abundances listed in table \ref{abs} for t$^2$
equal to zero, and a particular case of the first equation of this subsection
(see ecuation (15) of Peimbert et al., 2004, the particular case of their
ecuation (11)):

\begin{eqnarray}
\label{abunt2}
\lefteqn{\Big[\frac{N_{CEL}(X^{+i})}{N(H^{+})}\Big]_{t^2>0}\,=\,
  \frac{T(H\beta)^{-0.89}T(\lambda_{mn})^{0.5}}{T(\lambda_{mn}/\lambda_{m'n'}])^{-0.37}}
   } \nonumber\\ & & 
  {} \times\, exp\Big[-\frac{\Delta E}{k\,T(\lambda_{mn}/\lambda_{m'n'}])}+\frac{\Delta
  E}{k\,T(\lambda_{mn})}\Big]\,\times\, \Big[\frac{N_{CEL}(X^{+i})}{N_{RL}(H^{+})}\Big]_{t^2=0}
\end{eqnarray}

\noindent where $\Delta E$ is the energy difference, in eV, between the two
levels of the atomic transition that produces the line that we have used to
calculate the ionic abundace. 

\medskip 

Note that, for both schemes, from the calculated value for the chemical
abundances with t$^2$ greater than zero it is possible to interpolate or
extrapolate to derive the chemical abundances for other values of
t$^2$. Moreover, a variation in the temperatures used to derive the chemical
abundances  for t$^2$ equal to zero imply a modification for these abundances
and the value of t$^2$. However, the abundances calculated for t$^2$ greater
than zero not change, since the variations cancel each other
\cite{2004ApJS..150..431P}.

... poner cual es la tabla y demas....

%\newpage
%\hfill
%\newpage
\addcontentsline{toc}{section}{\numberline{}Bibliography}

\bibliographystyle{astron}
\bibliography{tesis}
